# Supplementary material for: Coupling of ferromagnetic and antiferromagnetic spin dynamics in Mn$_{2}$Au/NiFe thin-film bilayers
Source: arXiv:2302.07915 ancillary file (2023-02-15)
Supplement: Supplementary file 1 [file SI_Mn2Au-Py.pdf]

# Supplementary materials: Coupling of ferromagnetic and antiferromagnetic spin dynamics in $Mn_2Au$/NiFe thin-film bilayers

Hassan Al-Hamdo,[1,*] Tobias Wagner,[2] Yaryna Lytvynenko,[2,3] Gutenberg Kendzo,[1] Sonka Reimers,[2] Moritz Ruhwedel,[1] Misbah Yaqoob,[1] Vitaliy I. Vasyuchka,[1] Philipp Pirro,[1] Jairo Sinova,[2] Mathias Kläui,[2] Martin Jourdan,[2] Olena Gomonay,[2] and Mathias Weiler[1]

[1]*Fachbereich Physik and Landesforschungszentrum OPTIMAS, Rheinland-Pfälzische Technische Universität Kaiserslautern-Landau, 67663 Kaiserslautern, Germany*

[2]*Institute of Physics, Johannes Gutenberg-University Mainz, 55099 Mainz, Germany*

[3]*Institute of Magnetism of the NAS of Ukraine and MES of Ukraine, 03142 Kyiv, Ukraine*

## FABRICATION PROCESS

The samples consist of Ta(001)(13 nm)/$Mn_2$Au(001)(40 nm)/$Ni_{80}Fe_{20}$ (2 nm to 30 nm)/ /$SiN_x$(2 nm) heterostructures, which are prepared by rf magnetron sputtering on epiready $Al_2O_3$(r-plane) substrates. The Ta(001) buffer layers are sputtered with substrate temperatures of 700 °C. The epitaxial $Mn_2$Au(001) thin films are deposited at 500 °C and annealed at 700 °C for 75 minutes, as described in reference [1]. The polycrystalline $Ni_{80}Fe_{20}$ and the $SiN_x$ layers are deposited at room temperature. The $SiN_x$ layers are sputtered from a $Si_3N_4$ target and serve to prevent sample oxidation. The high quality of the $Mn_2$Au/$Ni_{80}Fe_{20}$ interface and the strong exchange coupling has been confirmed in reference [2].

## EXPERIMENTAL TECHNIQUES AND EVALUATION

To determine the resonance frequency of the uniform modes in the samples a 50-GHz /Keysight N5244A PNA) vector network analyzer is used. We use a coplanar waveguide (CPW) with a 80 µm wide center conductor and matched to 50 Ω, where the external magnetic field is swept in 5-mT steps and at each field all frequencies from 1 to 50 GHz are scanned. The VNA is used to generate and detect the rf signal up to 50 GHz. All measurements were done at a rf power of 5 dBm and at room temperature. By determining phase and amplitude of the microwave transmission $S_{21}$-parameter, we measured the absorption of rf power by the sample as a function of frequency. The utilized VNA-FMR spectrometer employs a magnet capable of applying fields up to 1.75 T in the sample plane. The external magnetic field values were recorded with a Hall-probe placed directly above the sample. The external magnetic field $\mu_0 H_0$ was varied from 1 T to 0 T. We remove the frequency-dependent background from our VNA-FMR measurements by calculating the normalized field derivative $d_\mathrm{D} S_{21}$ [3].

Following our earlier work [4] we start with the magnetic susceptibility composed of $N = 2$ Lorentzian resonance lines:

$$\chi = \sum_{i=1}^{N} \frac{A_i \exp(i\phi)}{f^2_{\mathrm{res}(i)} - f^2 - if\Delta f_i} \, , \tag{1}$$

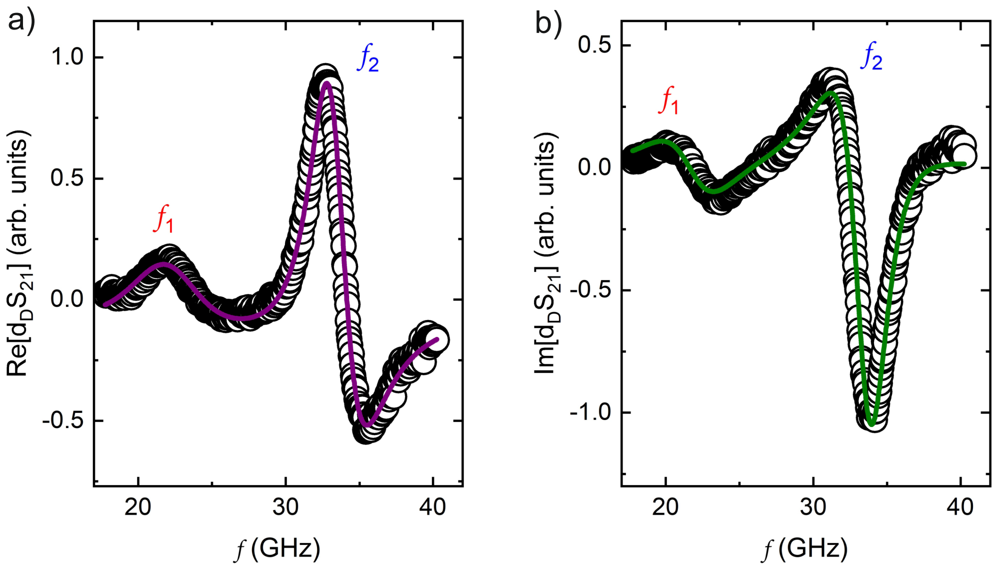


FIG. S1. (a), and (b) the real and imaginary part of of the measured susceptibility of the 5-nm sample obtained from transmission measurement ($S_{21}$) (black circles) for $\mu_0 H_0$= 100 mT with the complex susceptibility fit (solid lines) using Eq. (2), respectively.

which is then derived with respect to frequency:

$$\frac{\partial \chi}{\partial f} = C_0 + \sum_{i=1}^{N} \frac{A_i \exp(i\phi)}{f_{\mathrm{res}(i)}^2 - f^2 - if\Delta f_i} + A_i \exp(i\phi) f \frac{2f + i\Delta f_i}{(f_{\mathrm{res}(i)}^2 - f^2 - if\Delta f_i)^2}. \tag{2}$$

Here, $C_0$ accounts for the spurious background of real and imaginary parts, $A_i$ is the global amplitude of the $i$-th magnetic resonance, and $\Delta f_i$ is the full width at half maximum (FWHM) of the $i$-th magnetic resonance. We performed a global fit of the real and the imaginary part of the derivative divide data to Eq. (2) as shown in Figure S1 for data obtained at an external magnetic field $\mu_0 H_0 = 100\,\mathrm{mT}$ for the sample with 5nm-thick Py layer. The frequency resolution is 49 MHz as the number of points is 1001 in a range of 50 GHz. From such fits, we obtain the amplitudes $A_i$, resonance frequencies $f_{\mathrm{res}(i)}$ and linewidths $\Delta f_i$ as a function of $H_0$ for all samples. For all samples, the amplitude of $f_1$ is smaller than that of $f_2$, and the linewidth of $f_1$ is comparable to that of $f_2$ with both linewidths in the GHz range.

In Fig S2, we plotted the first (low frequency, $f_1$) and second (high frequency, $f_2$) resonance frequencies of the 4, 5, 7.5, 10-nm samples, and the second resonance frequency of 6, 15, and 30-nm samples as a function of external magnetic field (symbols). The lines are fits to Eq. (1) in the main text.

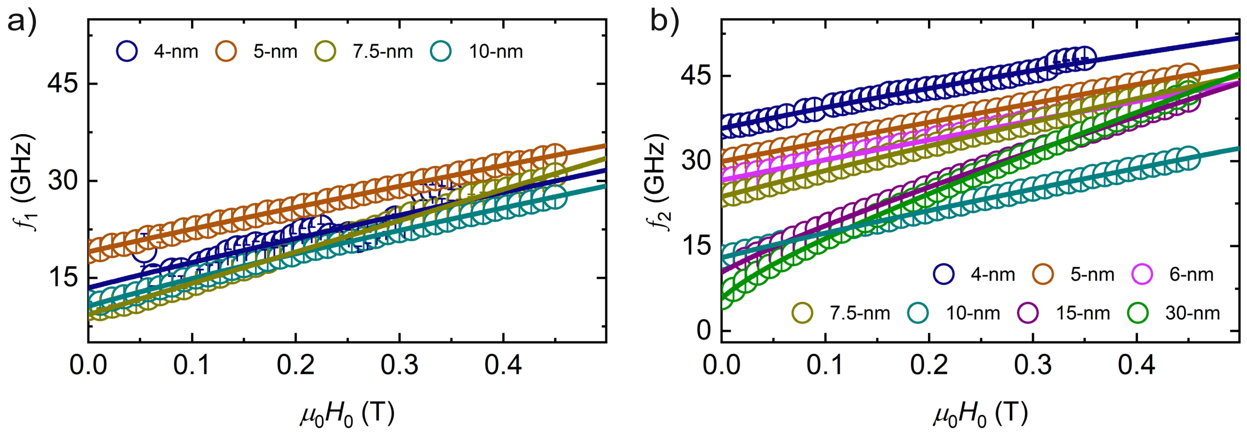


FIG. S2. (a), and (b) The first and second uniform modes of the 4-, 5-,10-nm, and 7.5-nm samples, and second uniform mode of the 6-, 15-, and 30-nm samples as a function of external magnetic field. Symbols are experimental data and the solid lines are fits to Eq. (1) from the main text.

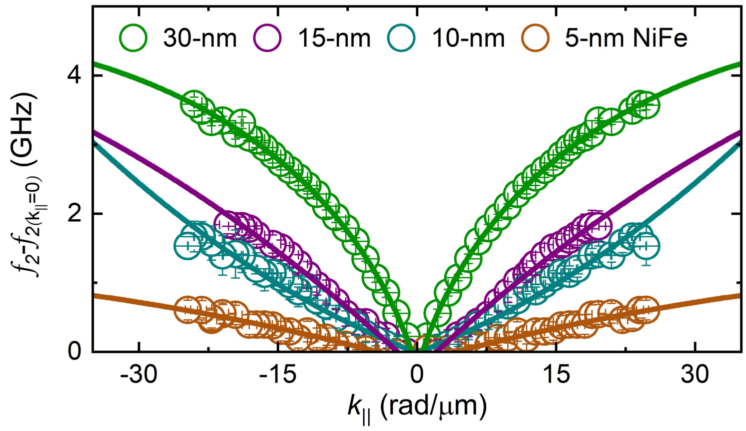


FIG. S3. The dispersion relation of the 5-,10-,15-,30-nm samples as a function of wave vector $k$, Symbols are experimental data and the solid lines are their fits with Eq.(1) from the main text.

Figure S3 shows the spin-wave dispersion relation of the 5, 10, 15, and 30-nm samples obtained based on wave-vector resolved BLS spectroscopy. The data is again fitted using Eq.(1) from the main text (solid lines). The measurements have been performed at an applied field of $\mu_0 H_0 = \pm 300$ mT, which is enough to switch the Néel vector of $Mn_2Au$ for all investigated Py thicknesses.

In Fig S4, the amplitudes $A_1$ and $A_2$ of first and second resonance frequency, respectively,

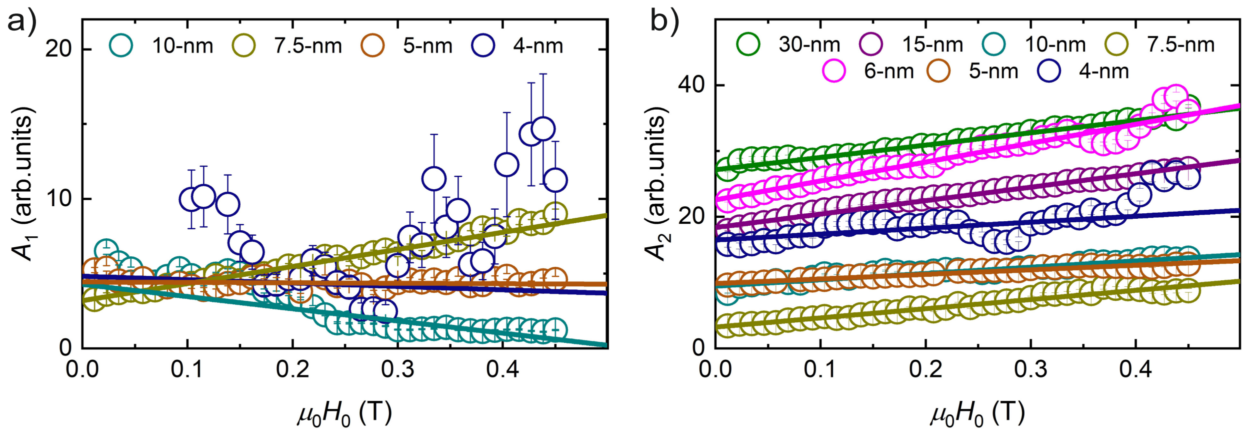


FIG. S4. The amplitudes $A_1$ of the first resonance frequency, and $A_2$ of second resonance frequency of all samples (colored circles). The solid lines are linear fits that demonstrate the general trend observed in the evolution of amplitudes with magnetic field.

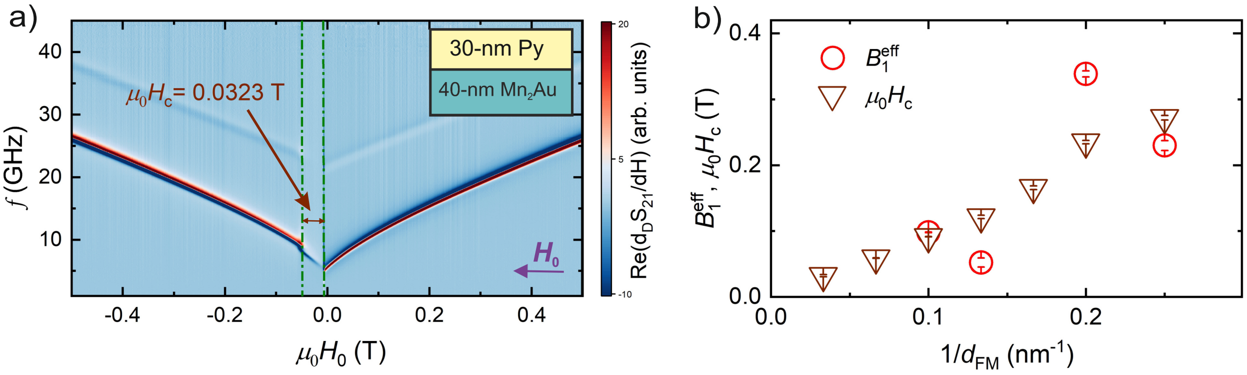


FIG. S5. (a) The coercive field $H_c$ is extracted from the FMR measurements. (b) The lower stiffness field, $B_1^{eff}$, and coercive field, $H_c$, as a function of inverted thickness of NiFe in $Mn_2Au$/NiFe bilayers.

are plotted as a function of the external magnetic field for all samples. We observe that the amplitudes increase with respect to the external magnetic field, and $A_2 > A_1$ for all samples, which indicates that the net precessing moment of the second mode is larger than that of the first mode.

## MODELING

We consider a bilayer antiferromagnetic-ferromagnetic (AFM-FM) system. The FM material is Permalloy, which we model using an isotropic distribution in the plane perpendicular

to the [001] axis in equilibrium. The AFM $Mn_2Au$ is modelled with tetragonal magnetic symmetry.

We neglect damping, the effect of an external field on the AFM and linearize the equations of motion:

$$\ddot{n}_y + \omega_{\parallel 0}^2 n_y - \tilde{c}^2 \Delta n_y = 0, \tag{3}$$

$$\ddot{n}_z + \omega_{\perp 0}^2 n_z - \tilde{c}^2 \Delta n_z = 0, \tag{4}$$

$$\dot{m}_y = \omega_{2,\mathrm{FM}} m_z - \gamma J_{\mathrm{FM}} \Delta m_z + \gamma \mu_0 H_0 m_z, \tag{5}$$

$$\dot{m}_z = -\omega_{1,\mathrm{FM}} m_y + \gamma J_{\mathrm{FM}} \Delta m_y - \gamma \mu_0 H_0 m_y, \tag{6}$$

where $\gamma$ is the gyromagnetic ratio of the electron, $\omega_{\parallel 0} \equiv 2\pi f_{\parallel 0}$, $\omega_{\perp 0} \equiv 2\pi f_{\perp 0}$ the AFM resonance frequencies and $\omega_{1,\mathrm{FM}} \equiv 2\pi f_{1,\mathrm{FM}}$, $\omega_{2,\mathrm{FM}} \equiv 2\pi f_{2,\mathrm{FM}}$, $\omega_{1,\mathrm{FM}} \ll \omega_{2,\mathrm{FM}}$ the FM resonance frequencies. $J_{\mathrm{FM}}$ and $H_0$ are as defined in the main text. We estimate the magnon velocity $\tilde{c} = 2\pi c$ with $c = \frac{\gamma}{2\pi}\sqrt{\frac{A_{\mathrm{AFM}} B_{\mathrm{ex}}}{M_{\mathrm{AFM}}}}$, where $A_{\mathrm{AFM}}$ is the AFM exchange stiffness, $B_{\mathrm{ex}}$ is the AFM exchange field and $M_{\mathrm{AFM}}$ is the AFM saturation magentization, as $\tilde{c} \approx 22.49\,\mathrm{km\,s^{-1}}$. Other values are given in Tab. S1.

We use the boundary conditions imposed on the system by the interlayer coupling to determine those FM magnons that are influenced by the coupling to the AFM layer. Without coupling, the boundary conditions at the surfaces of the FM layer are of *von-Neumann* type. When coupling to the AFM layer is included, the boundary condition at the interface is relaxed, such that the FM excitation can penetrate the interface:

$$z = \frac{d_{\mathrm{FM}}}{2}: \qquad J_{\mathrm{FM}} \partial_z m_y = 0,\ J_{\mathrm{FM}} \partial_z m_z = 0, \tag{7}$$

$$z = -\frac{d_{\mathrm{AFM}} + d_{\mathrm{FM}}}{2}: \qquad J_{\mathrm{AFM}} \partial_z n_y = 0,\ J_{\mathrm{AFM}} \partial_z n_z = 0, \tag{8}$$

$$z = -\frac{d_{\mathrm{FM}}}{2}: \qquad A_{\mathrm{FM}} \partial_z m_y + J_{\mathrm{exch}} \xi M_{\mathrm{FM}} M_{\mathrm{AFM}} \Big(n_y - m_y\Big) = 0, \tag{9}$$

$$A_{\mathrm{FM}} \partial_z m_z + J_{\mathrm{exch}} \xi M_{\mathrm{FM}} M_{\mathrm{AFM}} \Big(n_z - m_z\Big) = 0, \tag{10}$$

$$-A_{\mathrm{AFM}} \partial_z n_y + J_{\mathrm{exch}} \xi M_{\mathrm{FM}} M_{\mathrm{AFM}} \Big(m_y - n_y\Big) = 0, \tag{11}$$

$$-A_{\mathrm{AFM}} \partial_z n_z + J_{\mathrm{exch}} \xi M_{\mathrm{FM}} M_{\mathrm{AFM}} \Big(m_z - n_z\Big) = 0. \tag{12}$$

We parametrize the FM magnetisation and the AFM Néel vector as follows:

$$\mathbf{m}(z,\,t) \,=\, \hat{x} \,+\, \delta\mathbf{m}(z,\,t), \tag{13}$$

$$\delta\mathbf{m} \,=\, \begin{pmatrix} 0 \\ e^{i\,\omega_{1,\mathrm{FM}}\,t}\, m_y^{k_\parallel}(z) \\ e^{i\,\omega_{2,\mathrm{FM}}\,t}\, m_z^{k_{\perp\,\tau}}(z) \end{pmatrix}, \tag{14}$$

$$\mathbf{n}(z,\,t) \,=\, \hat{x} \,+\, \delta\mathbf{n}(z,\,t), \tag{15}$$

$$\delta\mathbf{n} \,=\, \begin{pmatrix} 0 \\ e^{i\,\omega_{\parallel\,0}\,t}\, n_y^{\kappa_1}(z) \\ e^{i\,\omega_{\perp\,0}\,t}\, n_z^{\kappa_2}(z) \end{pmatrix}. \tag{16}$$

The AFM Néel vector and the FM magnetisation equilibrate in-plane along the $x$ direction. We study out-of-plane oscillations perpendicular to this equilibrium orientation and restrict our study to the lowest energy mode. The wave vectors of the magnon modes are given for each component: $k_\parallel$, $k_{\perp\,\tau}$, $\kappa_1$ and $\kappa_2$; $\tau$ is either 1 or 2, depending on the mode coupling considered between the FM and the AFM. We assume that the coupling between the AFM and the FM layers concerns only the out-of-plane excitations of the FM, which is why we now focus on $k_{\perp,\,\tau}$.

When we consider a low energy excitation, we can assume evanescent modes in the AFM layer. That means, that while in the FM a magnonic mode is excited, the AFM is not excited. In this case, the oscillating magnons in the FM decay exponentially upon entering the AFM at the interface. We parametrise the perturbation as:

$$m_\alpha^k(z) \,=\, a_k\,\Big[e^{i\,k\,(z\,-\,d_{\mathrm{FM}}/2)} \,+\, e^{-i\,k\,(z\,-\,d_{\mathrm{FM}}/2)}\Big], \tag{17}$$

$$n_\alpha^\kappa(z) \,=\, c_\kappa\,\Big[e^{\kappa\,(z\,+\,d_{\mathrm{FM}}\,/\,2)} \,+\, e^{-\kappa\,(z\,+\,d_{\mathrm{FM}}\,/\,2)}\Big]. \tag{18}$$

Here, $a_\mathbf{k}$ and $c_\kappa$ denote the coefficients of the perturbation to the order parameter. $\alpha$ denote the spatial components and $k$ and $\kappa$ have to be replaced by the wave vectors defined in Eqn. (18) according to the spatial component under consideration. From the solution obtained below, we can estimate the amplitudes in the FM and the AFM for the case of no coupling $J_{\mathrm{exch}} = 0$, and the two coupled modes for non-zero coupling. We show these results in Fig. S6.

By inserting the ansatz Eqns. (17), (18) into the boundary conditions Eqns. (7), (8), (9),

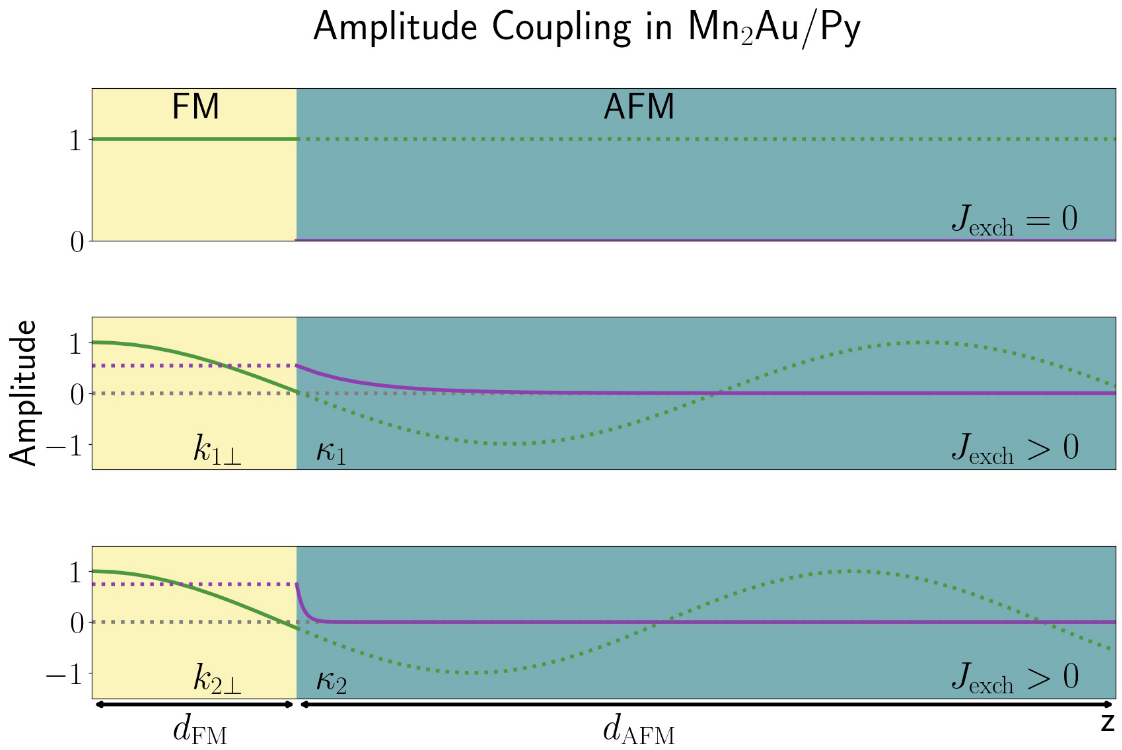


FIG. S6. In the case of no coupling $J_{\mathrm{exch}} = 0$ the amplitude of the resonance mode in the FM is constant, and no resonance mode is present in the AFM (upper panel). For non-zero coupling, the excitation in the FM leads to an evanescent mode in the AFM. Both resonance modes corresponding to $k_{1\perp}$, $\kappa_1$ and $k_{1\perp}$, $\kappa_1$ are shown, respectively (middle and lower panel).

(10), (11), (12), we obtain for the boundary condition on the wave vectors at $z = -d_{\mathrm{FM}}/2$:

$$\Big[A_{\mathrm{FM}}\, k_{\perp\tau} \sin(k_{\perp\tau}\, d_{\mathrm{FM}}) - J_{\mathrm{exch}}\, M_{\mathrm{FM}}\, M_{\mathrm{AFM}}\, \xi \cos(k_{\perp\tau}\, d_{\mathrm{FM}})\Big]\, a + J_{\mathrm{exch}}\, M_{\mathrm{FM}}\, M_{\mathrm{AFM}}\, \xi \cosh(\kappa_\tau\, d_{\mathrm{AFM}})\, c = 0, \tag{19}$$

$$J_{\mathrm{exch}}\, M_{\mathrm{FM}}\, M_{\mathrm{AFM}}\, \xi \cos(k_{\perp\tau}\, d_{\mathrm{FM}})\, a + \Big[- A_{\mathrm{AFM}}\, \kappa \sinh(\kappa_\tau\, d_{\mathrm{AFM}}) - J_{\mathrm{exch}}\, M_{\mathrm{FM}}\, M_{\mathrm{AFM}}\, \xi \cosh(\kappa_\tau\, d_{\mathrm{AFM}})\Big]\, c = 0, \tag{20}$$

from which we extract a condition on $k_{\perp\tau}$:

$$- A_{\mathrm{FM}}\, A_{\mathrm{AFM}}\, k_{\perp\tau}\, \kappa_\tau \sin(k_{\perp\tau}\, d_{\mathrm{FM}}) \sinh(\kappa_\tau\, d_{\mathrm{AFM}}) - A_{\mathrm{FM}}\, k_{\perp\tau} \sin(k_{\perp\tau}\, d_{\mathrm{FM}})\, J_{\mathrm{exch}}\, M_{\mathrm{FM}}\, M_{\mathrm{AFM}}\, \xi \cosh(\kappa_\tau\, d_{\mathrm{AFM}}) + A_{\mathrm{AFM}}\, \kappa_\tau \sinh(\kappa_\tau\, d_{\mathrm{AFM}})\, J_{\mathrm{exch}}\, M_{\mathrm{FM}}\, M_{\mathrm{AFM}}\, \xi \cos(k_{\perp\tau}\, d_{\mathrm{FM}}) = 0. \tag{21}$$

We approximate the AFM wave vector ($f \ll f_{\|0}$):

$$\begin{aligned}
\kappa_1 &= \frac{\sqrt{f_{\|0}^2 - f^2}}{c} \approx \frac{\sqrt{f_{\|0}^2}}{c}, \\
\kappa_2 &= \frac{\sqrt{f_{\perp 0}^2 - f^2}}{c} \approx \frac{\sqrt{f_{\perp 0}^2}}{c}.
\end{aligned} \tag{22}$$

With the relation between the resonance frequencies and the AFM wave vectors we can simplify the condition on $k_{\perp 1/2}$:

$$\begin{aligned}
&k_{\perp \tau}\, \kappa_\tau \tan(k_{\perp \tau}\, d_{\mathrm{FM}}) \tanh(\kappa_\tau\, d_{\mathrm{AFM}}) \\
&= \frac{J_{\mathrm{exch}}\, \xi}{J_{\mathrm{FM}}\, J_{\mathrm{AFM}}} \Big[ -\, A_{\mathrm{FM}}\, k_{\perp \tau} \tan(k_{\perp \tau}\, d_{\mathrm{FM}}) \,+\, A_{\mathrm{AFM}}\, \kappa_\tau \tanh(\kappa_\tau\, d_{\mathrm{AFM}}) \Big],
\end{aligned} \tag{23}$$

$$\begin{aligned}
\Rightarrow \quad &k_{\perp 1/2}\, \frac{f_{\|0\,/\perp 0}}{c} \tan(k_{\perp 1/2}\, d_{\mathrm{FM}}) \tanh\Big(\frac{f_{\|0\,/\perp 0}}{c}\, d_{\mathrm{AFM}}\Big) \\
&= \frac{J_{\mathrm{exch}}\, \xi}{J_{\mathrm{FM}}\, J_{\mathrm{AFM}}} \Big[ -\, A_{\mathrm{FM}}\, k_{\perp 1/2} \tan(k_{\perp 1/2}\, d_{\mathrm{FM}}) \\
&\quad +\, A_{\mathrm{AFM}}\, \frac{f_{\|0\,/\perp 0}}{c} \tanh\Big(\frac{f_{\|0\,/\perp 0}}{c}\, d_{\mathrm{AFM}}\Big) \Big]
\end{aligned} \tag{24}$$

These relations are not solvable analytically, which is why we solve them graphically. For this we rewrite:

$$k_{\perp 1/2}\, d_{\mathrm{FM}} \tan(k_{\perp 1/2}\, d_{\mathrm{FM}}) = \frac{\frac{J_{\mathrm{exch}}\, M_{\mathrm{AFM}}\, \xi}{A_{\mathrm{FM}}}\, d_{\mathrm{FM}}\, \frac{f_{\|0\,/\perp 0}}{c} \tanh\Big(\frac{f_{\|0\,/\perp 0}}{c}\, d_{\mathrm{AFM}}\Big)}{\frac{f_{\|0\,/\perp 0}}{c} \tanh\Big(\frac{f_{\|0\,/\perp 0}}{c}\, d_{\mathrm{AFM}}\Big) + \frac{J_{\mathrm{exch}}\, M_{\mathrm{FM}}\, \xi}{A_{\mathrm{AFM}}}}. \tag{25}$$

For the parameter values of this experiment, we can approximate $\tan(x) \approx x$, $M_{\mathrm{AFM}} \approx M_{\mathrm{FM}}$ and $\tanh(x) \approx 1$:

$$k_{\perp 1/2} = \sqrt{\frac{1}{A_{\mathrm{FM}}}\, \frac{J_{\mathrm{exch}}\, \xi\, A_{\mathrm{AFM}}\, \kappa_{1,2}}{\frac{J_{\mathrm{AFM}}}{M_{\mathrm{FM}}}\, \kappa_{1,2} + J_{\mathrm{exch}}\, \xi}}\, \frac{1}{\sqrt{d_{\mathrm{FM}}}}. \tag{26}$$

The wave vector of the FM excitation is modified by the interlayer coupling: The easy-plane AFM possesses two non-degenerate resonance modes and FM modes can couple to each of them, given a suitable combination of AFM and FM wave vectors. The coupling between the AFM and the FM layer leads to a modification of the FM magnon frequency in which the presence of the AFM layer acts as an effective anisotropy to the FM. This leads to a splitting of the FM mode into two branches: a higher frequency branch and a lower frequency branch. Not only increases the FM resonance mode due to the effective anisotropy, but also two resonance modes emerge, rather than one in the case of a pure FM system. The parameters used in this theoretical work are given in Tab. S1.

| Parameter | Value | Reference |
|---|---|---|
| $M_{\mathrm{FM}}$ | $8.6 \cdot 10^5\,\frac{\mathrm{A}}{\mathrm{m}}$ | [5] |
| $A_{\mathrm{FM}}$ | $10.0\,\frac{\mathrm{pJ}}{\mathrm{m}}$ | [6] |
| $M_{\mathrm{AFM}}$ | $1.6 \cdot 10^6\,\frac{\mathrm{A}}{\mathrm{m}}$ | [7] |
| $A_{\mathrm{AFM}}$ | $20.1\,\frac{\mathrm{pJ}}{\mathrm{m}}$ | [7, 8] |
| $B_{\mathrm{ex}}$ | $1300\,\mathrm{T}$ | [9] |
| $f_{\parallel 0}$ | $0.3\,\mathrm{THz}$ | This work |
| $f_{\perp 0}$ | $> 1\,\mathrm{THz}$ | This work |
| $\kappa_1$ | $0.09\,\frac{1}{\mathrm{nm}}$ | This work |
| $\kappa_2$ | $\gg \kappa_1$ | This work |
| $J_{\mathrm{exch}}\,M_{\mathrm{AFM}}\,\xi$ | $1.6\,\mathrm{T\,nm}$ | This work |

TABLE S1. Used literature values and parameters determined from our analysis.

* E-Mail: alhamdo@rhrk.uni-kl.de

[1] M. Jourdan, H. Bräuning, A. Sapozhnik, H.-J. Elmers, H. Zabel, and M. Kläui, J. Phys. D: Appl. Phys. **48**, 385001 (2015).

[2] S. P. Bommanaboyena, D. Backes, L. S. I. Veiga, S. S. Dhesi, Y. R. Niu, B. Sarpi, T. Denneulin, A. Kovács, and M. Jourdan, Nat. Commun. **12**, 6539 (2021).

[3] H. Maier-Flaig, S. T. B. Goennenwein, R. Ohshima, M. Shiraishi, R. Gross, H. Huebl, and M. Weiler, Rev. Sci. Instrum. **89**, 076101 (2018).

[4] M. Weiler, A. Aqeel, M. Mostovoy, A. Leonov, S. Geprägs, R. Gross, H. Huebl, T. T. M. Palstra, and S. T. B. Goennenwein, Phys. Rev. Lett. **119**, 237204 (2017).

[5] G. Nahrwold, J. M. Scholtyssek, S. Motl-Ziegler, O. Albrecht, U. Merkt, and G. Meier, J. Appl. Phys. **108**, 013907 (2010).

[6] N. Smith, D. Markham, and D. LaTourette, J. of Appl. Phys. **65**, 4362 (1998).

[7] A. A. Sapozhnik, M. Filianina, S. Y. Bodnar, A. Lamirand, M.-A. Mawass, Y. Skourski, H.-J. Elmers, H. Zabel, M. Kläui, and M. Jourdan, Phys. Rev. B **97**, 134429 (2018).

[8] S. Khmelevskyi and P. Mohn, Appl. Phys. Lett. **93**, 162503 (2008).

[9] V. Barthem, C. Colin, H. Mayaffre, M. Julien, and D. Givord, Nat. Commun. **4**, 2892 (2013).
